# Supplementary material for: DC4CR: When Cloud Removal Meets Diffusion Control in Remote Sensing
Source: arXiv:2504.14785 source file (2025-05-10)
Supplement: Supplementary file 1 [file X_suppl.tex]

\clearpage
\setcounter{page}{1}
\setcounter{table}{0}
\setcounter{figure}{0}

\appendix
% \section{Appendix}
\label{sec:appendix}
% \begin{appendices}

% 设置编号
\setcounter{table}{0}   
\setcounter{figure}{0}
\setcounter{section}{0}
\setcounter{equation}{0}

\section{Figures and Tables}
\label{sec_A2}
This section includes:

\begin{enumerate}
    \item Models comparison results (Figure \ref{fig:model_compare_full});

    % \item Comparison of weighting scalling factor \(\alpha\) settings (Figure \ref{fig:lora_compare_imgs});
    
    \item $k$-Means clustering results to the dataset (Figure \ref{fig:groups});
    
    % \item $k$-means clustering statistics of datasets (Table \ref{table:progressive_data});
    
    % \item Weight scalling factor \(\alpha\) settings results (Table \ref{table:lora_alpha});
    
    \item Enhancement parameters selection results (Figure \ref{fig:params_freeu}).
\end{enumerate}

% appendix fig A1
% fig:model_compare_full
\begin{figure*}[!htb] % h, t, b
    \centering
    \includegraphics[width=1.0\linewidth]{figs/model_imgs_3.pdf} 
    \caption{Models comparison results. It indicates that the DC4CR excels across all models, showing significant advantages, particularly in handling complex datasets.}
    \label{fig:model_compare_full}
\end{figure*}

% appendix fig A2
% fig:lora_compare_imgs
% \begin{figure*}[!htb] % h, t, b
%     \centering
%     \includegraphics[width=0.86\linewidth]{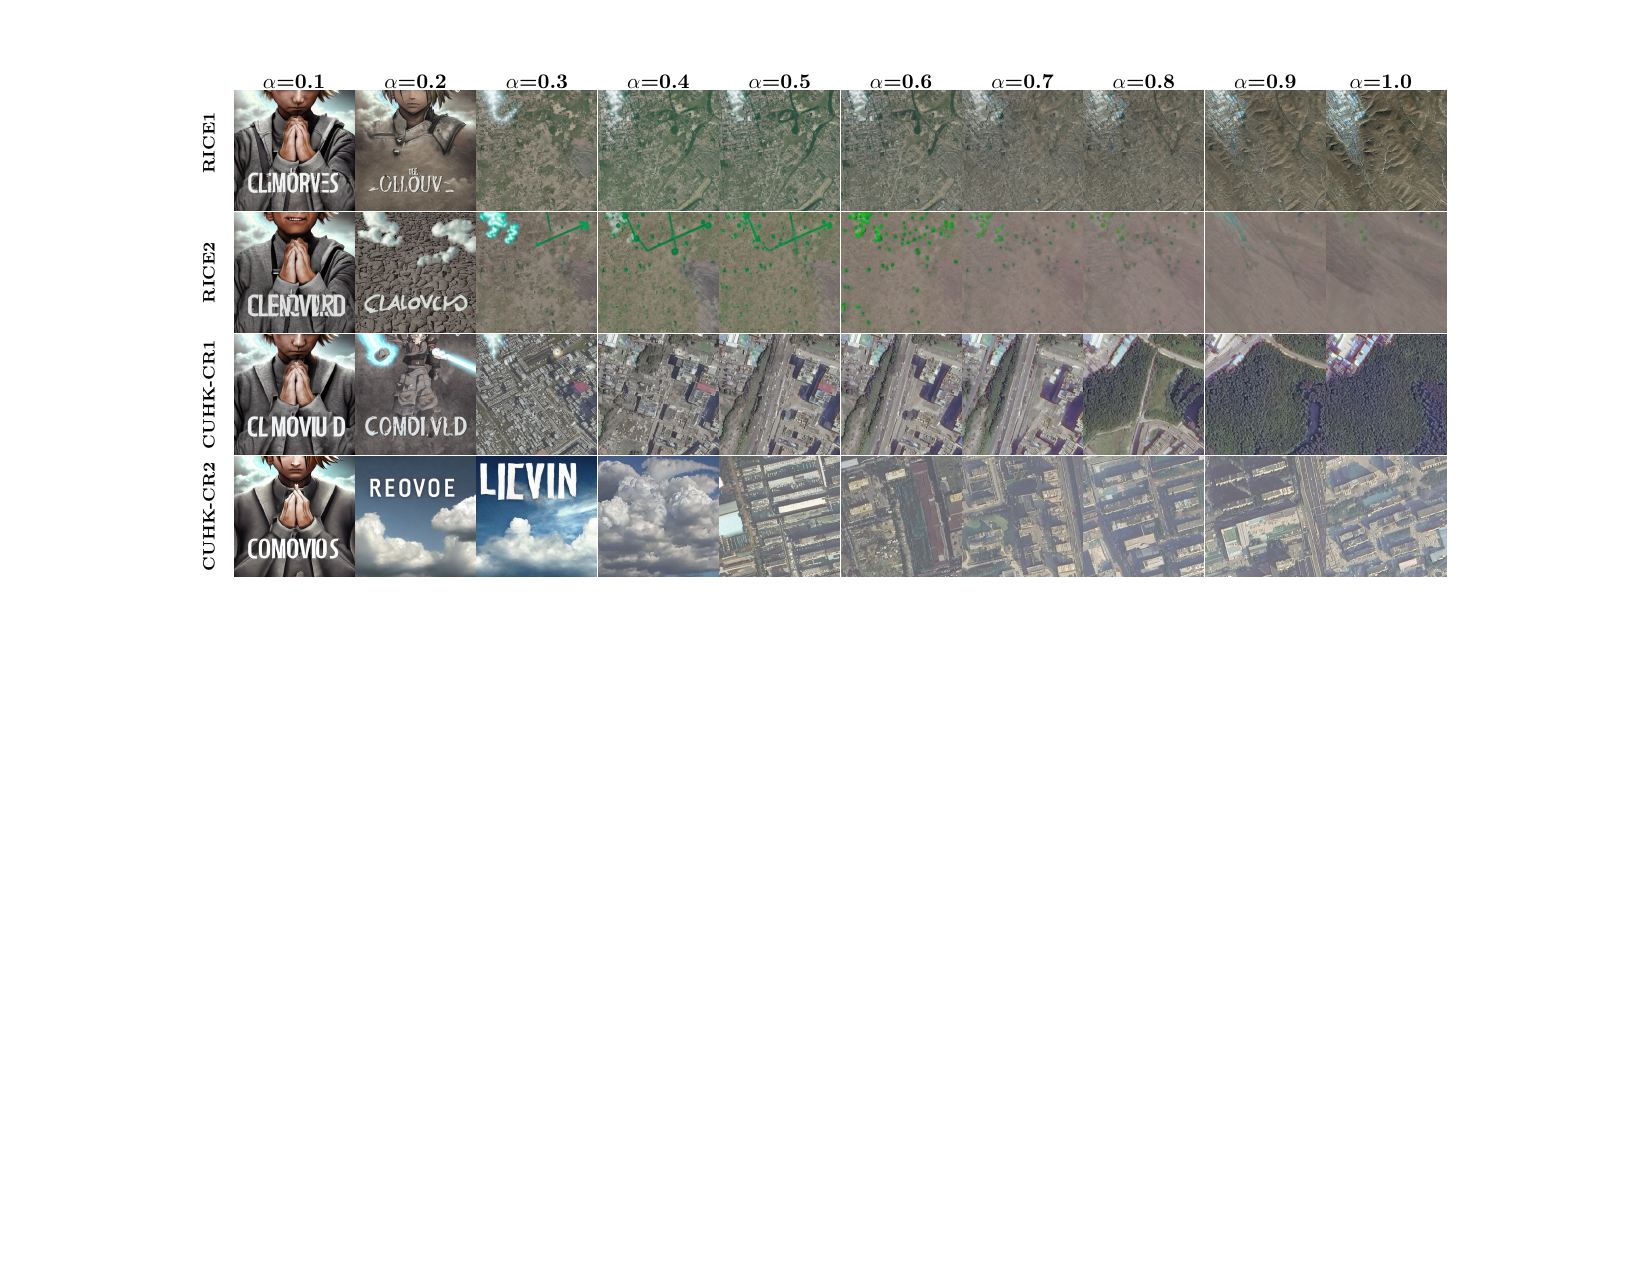} 
%     \caption{Comparison of weighting scalling factor \(\alpha\) settings. It demonstrates that \(\alpha\) values greater than 0.5 lead to better outcomes, with higher values resulting in clearer and more detailed images. This trend highlights the importance of selecting appropriate \(\alpha\) settings to optimize image quality.}
%     \label{fig:lora_compare_imgs}
% \end{figure*}

% appendix fig A3 -> A2
% fig:groups
\begin{figure*}[!htb] % h, t, b
    \centering
    \includegraphics[width=0.49\linewidth]{figs/mse_result_RICE1_k2.pdf} 
    \includegraphics[width=0.49\linewidth]{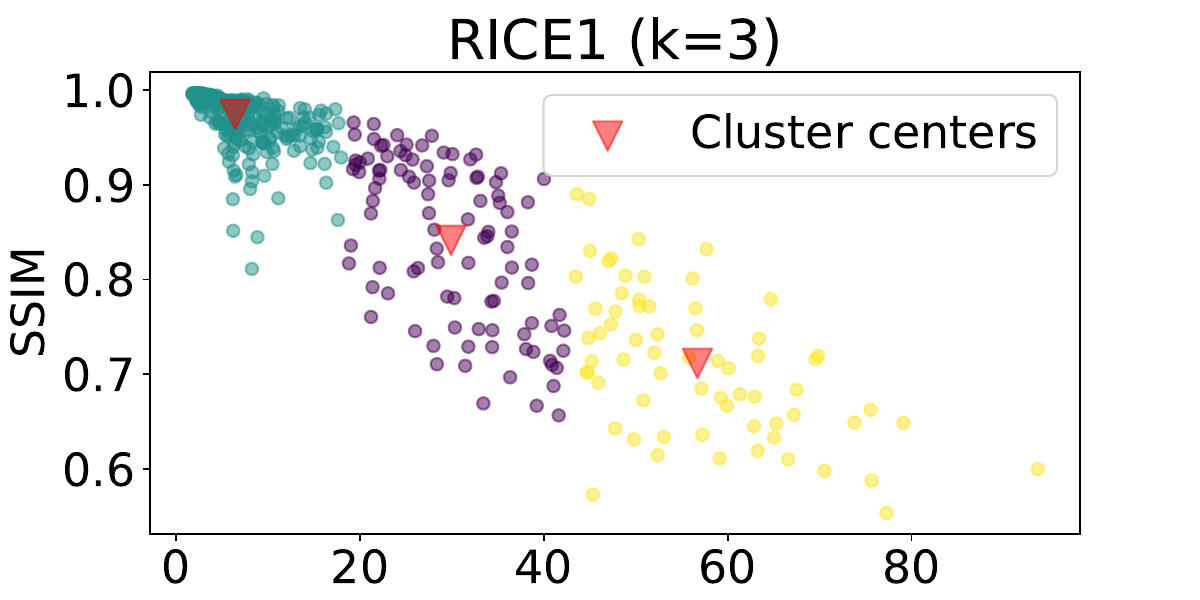} 
    \includegraphics[width=0.49\linewidth]{figs/mse_result_RICE2_k2.pdf} 
    \includegraphics[width=0.49\linewidth]{figs/mse_result_RICE2_k3.pdf} 
    \includegraphics[width=0.49\linewidth]{figs/mse_result_CUHK-CR1_k2.pdf} 
    \includegraphics[width=0.49\linewidth]{figs/mse_result_CUHK-CR1_k3.pdf} 
    \includegraphics[width=0.49\linewidth]{figs/mse_result_CUHK-CR2_k2.pdf} 
    \includegraphics[width=0.49\linewidth]{figs/mse_result_CUHK-CR2_k3.pdf} 
    \caption{$k$-Means clustering results to the dataset. It shows the cluster centers and the data distribution within each cluster. The visualization highlights the spatial arrangement and density, providing insights into the underlying structure and characteristics of the dataset.}
    \label{fig:groups}
\end{figure*}

\begin{figure*}[!ht] % h, t, b
    \centering
    \includegraphics[width=0.49\linewidth]{figs/result_sd_freeu_compare_RICE1_b1.pdf} 
    \includegraphics[width=0.49\linewidth]{figs/result_sd_freeu_compare_RICE1_b2.pdf} 
    \includegraphics[width=0.49\linewidth]{figs/result_sd_freeu_compare_RICE1_s1.pdf} 
    \includegraphics[width=0.49\linewidth]{figs/result_sd_freeu_compare_RICE1_s2.pdf} 
    \caption{Enhancement parameters selection results. It illustrates the impact of varying parameters \(s_1\), \(s_2\), \(b_1\), and \(b_2\) on model performance. The analysis identifies the optimal parameter values as \(s_1 = 0.9\), \(s_2 = 0.4\), \(b_1 = 1.1\), and \(b_2 = 1.1\), which provide the best balance between model accuracy and image quality.}
    \label{fig:params_freeu}
\end{figure*}
